# Supplementary material for: Offset-free Model Predictive Control: A Ball Catching Application with a Spherical Soft Robotic Arm
Source: arXiv:2103.07379 source file (2021-03-12)
Supplement: Supplementary file 1 [file appendix.tex]

% !TEX root = ../root.tex
\section*{Appendix}
